# Supplementary material for: The $N_f=2$ QCD chiral phase transition with Wilson fermions at zero and imaginary chemical potential
Source: arXiv:1602.06129 source file (2016-11-08)
Supplement: Supplementary file 1 [file appendix.tex]

\appendix
\section{Simulation details}
\label{ch:appendix}
